# Supplementary material for: Mechanizing Refinement Types (extended)
Source: arXiv:2207.05617 source file (2022-07-12)
Supplement: Supplementary file 1 [file supplementary.tex]

\documentclass[acmsmall,review,anonymous]{acmart}\settopmatter{printfolios=true,printccs=false,printacmref=false}
\settopmatter{printacmref=false} % Removes citation information below abstract
\renewcommand\footnotetextcopyrightpermission[1]{} % removes footnote with conference information in first column
\setcopyright{none}

%% Uncomment the following line to make margin \mynote s disappear
% \def\dbg{false}

\usepackage{booktabs}   %% For formal tables:
                        %% http://ctan.org/pkg/booktabs
\usepackage{subcaption} %% For complex figures with subfigures/subcaptions
                        %% http://ctan.org/pkg/subcaption

\bibliographystyle{ACM-Reference-Format.bst}
% \citestyle{acmauthoryear}
%\bibliographystyle{plain}

\usepackage{float}
\usepackage[english]{babel}

\usepackage[T1]{fontenc}
\usepackage[scaled=0.85]{beramono}

\usepackage{todonotes}

% \usepackage{fixme}
% \fxsetup{layout={inline}}
% % COMMENT THE FOLLOWING LINE TO REMOVE TODOS
% \fxsetup{draft}

\usepackage{framed}
\usepackage{hyperref}
\usepackage{xspace}
\usepackage{fancyvrb}
\usepackage{listings}
\usepackage{booktabs}
\hypersetup{colorlinks=true,allcolors=blue}
\usepackage{array}%, bigfoot}
\usepackage{url}
\usepackage{comment}
\usepackage{pifont}

\usepackage{stmaryrd}
\usepackage{xcolor}
\usepackage{mathtools}
\usepackage{xspace}
\usepackage{mathpartir}
\usepackage{graphicx}
\usepackage{caption}
\usepackage{xcolor}
\usepackage{tikz}
\usetikzlibrary{arrows.meta,automata,shapes}
\input{haskellListings}
\usepackage{semantic}
\usepackage{float}
\usepackage{commands_full}
\usepackage[shortcuts]{extdash}
\usepackage{cleveref}
\usepackage{enumitem}

\makeatother

\lstset{
    keywordstyle=\color{blue}
  , basicstyle=\ttfamily
  , commentstyle={}
  , columns=flexible
  %, numbers=left
  , showstringspaces=false
  }

\title{Mechanizing Refinements with Types}
% \subtitle{A fun subtitle}

\author{Michael Borkowski}
\affiliation{\institution{UC San Diego} \country{USA}}
\email{mborkows@eng.ucsd.edu}

\author{Niki Vazou}
\affiliation{\institution{IMDEA} \country{Spain}}
\email{niki.vazou@imdea.org}

\author{Ranjit Jhala}
\affiliation{\institution{UC San Diego} \country{USA}}
\email{rjhala@eng.ucsd.edu}

\begin{document}
%\pgfdeclarelayer{background}
%\pgfdeclarelayer{middleground}
%\pgfdeclarelayer{foreground}
%\pgfsetlayers{background,middleground,main,foreground}

\maketitle

\appendix
\input{aa-proofs}
\input{ab-proofs}

\end{document}
